# Supplementary material for: DeepEye-SQL: A Software-Engineering-Inspired Text-to-SQL Framework
Source: arXiv:2510.17586 source file (2026-04-03)
Supplement: Supplementary file 1 [file appendix.tex]

\clearpage
\onecolumn
\appendix

\section{Prompt Templates in \model}
\label{sec:appendix_prompts}

\subsection{Keyword Extraction Prompt}
\label{subsec:prompt_keyword_extraction}

This prompt is used in the \textit{Online Retrieval} stage of the \textit{Semantic Value Retrieval} phase. Its objective is to instruct the LLM to analyze the user's question and any available hints to extract a list of keywords, keyphrases, and named entities that are likely to be relevant for filtering values in a \texttt{WHERE} clause.

\begin{lstlisting}[
    frame=single,
    caption={Keyword Extraction Prompt},
    label={lst:keyword_extraction},
    basicstyle=\ttfamily\small,
    breaklines=true
]
Objective: Analyze the given question and hint to identify and extract keywords, keyphrases, and named entities. These elements are crucial for understanding the core components of the inquiry and the guidance provided. This process involves recognizing and isolating significant terms and phrases that could be instrumental in formulating searches or queries related to the posed question.

Instructions:
Read the Question Carefully: Understand the primary focus and specific details of the question. Look for any named entities (such as organizations, locations, etc.), technical terms, and other phrases that encapsulate important aspects of the inquiry.

Analyze the Hint: The hint is designed to direct attention toward certain elements relevant to answering the question. Extract any keywords, phrases, or named entities that could provide further clarity or direction in formulating an answer.

List Keyphrases and Entities: Combine your findings from both the question and the hint into a single Python list. This list should contain:
- Keywords: Single words that capture essential aspects of the question or hint.
- Keyphrases: Short phrases or named entities that represent specific concepts, locations, organizations, or other significant details.

Ensure to maintain the original phrasing or terminology used in the question and hint.

Example 1:
Question: What is the annual revenue of Acme Corp in the United States for 2022?
Hint: Focus on financial reports and U.S. market performance for the fiscal year 2022.

<result>
["annual revenue", "Acme Corp", "United States", "2022", "financial reports", "U.S. market performance", "fiscal year"]
</result>

Example 2:
Question: In the Winter and Summer Olympics of 1988, which game has the most number of competitors? Find the difference of the number of competitors between the two games.
Hint: the most number of competitors refer to MAX(COUNT(person_id)); SUBTRACT(COUNT(person_id where games_name = '1988 Summer'), COUNT(person_id where games_name = '1988 Winter'));

<result>
["Winter Olympics", "Summer Olympics", "1988", "1988 Summer", "Summer", "1988 Winter", "Winter"]
</result>

Example 3:
Question: How many Men's 200 Metres Freestyle events did Ian James Thorpe compete in?
Hint: Men's 200 Metres Freestyle events refer to event_name = 'Swimming Men''s 200 metres Freestyle'; events compete in refers to event_id;

<result>
["Swimming Men's 200 metres Freestyle", "Ian James Thorpe", "Ian", "James", "Thorpe"]
</result>

Task:
Given the following question and hint, identify and list all relevant keywords, keyphrases, and named entities.

Question: {QUESTION}
Hint: {HINT}

Output only the following XML format (no explanations), ensure the list is a valid Python list:

<result>
[your_keywords_python_list]
</result>
\end{lstlisting}

\clearpage
\subsection{Direct Schema Linking Prompt}
\label{subsec:prompt_direct_linking}

This prompt corresponds to the \textit{Direct Schema Linking} strategy within the \textit{Robust Schema Linking} phase. It instructs the LLM to act as a data analyst, explicitly identifying and reasoning about the necessary tables and columns based on the schema, question, and retrieved value examples.

\begin{lstlisting}[
    frame=single,
    caption={Direct Schema Linking Prompt},
    label={lst:direct_linking},
    basicstyle=\ttfamily\small,
    breaklines=true
]
# Task:
You are an expert and very smart data analyst.
Your task is to examine the provided database schema, understand the posed question, and use the hint to **pinpoint the specific tables and columns** that are essential for crafting a SQL query to answer the question.

# Instructions:
The given schema provides a detailed definition of the database's structure, including tables, their columns, primary keys, foreign keys, and any relevant details about relationships or constraints.
The given hint aims to direct your focus towards the specific elements of the database schema that are crucial for answering the question effectively.

For each of the selected tables and columns, explain why exactly it is necessary for answering the question. Your reasoning should be concise and clear, demonstrating a logical connection between the selected items and the question asked.

[IMPORTANT!]
1. For key phrases mentioned in the question, we have provided the most similar values within the columns (TEXT-TYPE columns) denoted by "Value Examples". **This is a critical hint to identify the tables/columns that will be used in the SQL query.**
2. If you are not sure whether a column is needed or not, it's better to include it in your selection. **It's safer to select more columns than to miss necessary ones.**
3. If a column contains values that are related to the current question (check the "Value Examples"), you MUST include this column in your selection.
4. If there are multiple tables to JOIN, you MUST ensure that the joined tables have EXPLICIT FOREIGN KEYS between them. For example, "TableA -> TableB, TableC -> TableB", directly join TableA and TableC is NOT ALLOWED, you must join TableA and TableB, and then join TableB and TableC.

# Output Format:
Please respond with XML code structured as follows:
<reasoning>
    Your reasoning for selecting the tables and columns, be concise and clear.
</reasoning>
<result>
    <table table_name="table_name">
        <column column_name="column_name" />
        ...
    </table>
    <table table_name="another_table_name">
        <column column_name="another_column_name" />
        ...
    </table>
    ...
</result>

# Input:
## Database Schema:
{DATABASE_SCHEMA}

## Question:
{QUESTION}

## Hint:
{HINT}

Only output the XML code following the output format as your response.

# Output:
\end{lstlisting}

\clearpage
\subsection{Divide-and-Conquer SQL Generation Prompt}
\label{subsec:prompt_dc_sql}

This prompt guides the \textit{Divide-and-Conquer-based SQL Generator}. It instructs the LLM to recursively break down a complex question into simpler sub-questions, solve them, and then reassemble the resulting SQL fragments into a final, complete query.

\begin{lstlisting}[
    frame=single,
    caption={Divide-and-Conquer SQL Generation Prompt},
    label={lst:dc_sql},
    basicstyle=\ttfamily\small,
    breaklines=true
]
# Task:
You are an experienced database expert.
You will be given details about the database schema and you need understand the tables and columns.
Then you need to generate a SQL query given the database information, a question and some additional information.

# Instructions:
You will be using a way called "recursive divide-and-conquer approach to SQL query generation from natural language".

Here is a high level description of the steps.
1. **Divide (Decompose Sub-question with Pseudo SQL):** The complex natural language question is recursively broken down into simpler sub-questions. Each sub-question targets a specific piece of information or logic required for the final SQL query. 
2. **Conquer (Real SQL for sub-questions):** For each sub-question (and the main question initially), a "pseudo-SQL" fragment is formulated. This pseudo-SQL represents the intended SQL logic but might have placeholders for answers to the decomposed sub-questions. 
3. **Combine (Reassemble):** Once all sub-questions are resolved and their corresponding SQL fragments are generated, the process reverses. The SQL fragments are recursively combined by replacing the placeholders in the pseudo-SQL with the actual generated SQL from the lower levels.
4. **Final Output:** This bottom-up assembly culminates in the complete and correct SQL query that answers the original complex question.

# Important Rules:
1. **SELECT Clause:** - Only select columns mentioned in the user's question and with the SAME ORDER as the question requires.
    - Avoid unnecessary columns or values.
2. **Handling NULLs:**
    - If a column may contain NULL values, use `JOIN` or `WHERE <column> IS NOT NULL`.
3. **FROM/JOIN Clauses:**
    - Only include tables essential to answer the question.
4. **Thorough Question Analysis:**
    - Address all conditions mentioned in the question.
5. **DISTINCT Keyword:**
    - Use `SELECT DISTINCT` when the question requires unique values (e.g., IDs, URLs). 
    - Refer to column statistics ("Total count" and "Distinct count") to determine if `DISTINCT` is necessary.
6. **Column Selection:**
    - Carefully analyze column descriptions and hints to choose the correct column when similar columns exist across tables.
7. **String Concatenation:**
    - Never use `|| ' ' ||` or any other method to concatenate strings in the `SELECT` clause.
8. **JOIN Preference:**
    - Prioritize `INNER JOIN` over nested `SELECT` statements.
9. **SQLite Functions Only:**
    - Use only functions available in SQLite.
10. **Date Processing:**
    - Utilize `STRFTIME()` for date manipulation (e.g., `STRFTIME('%Y', SOMETIME)` to extract the year).
11. **Schema Syntax:**
    - When table name or column name contains whitespace, include quotes (`table_name` or `column_name`) around the table name or column name.
12. **Value Examples:**
    - For key phrases mentioned in the question, we have provided the most similar values within the columns (TEXT-TYPE columns) denoted by "Value Examples".
13. **Foreign Key Constraints:**
    - If there are multiple tables to JOIN, you MUST ensure that the joined tables have EXPLICIT FOREIGN KEYS between them. For example, "TableA -> TableB, TableC -> TableB", directly join TableA and TableC is NOT ALLOWED, you must join TableA and TableB, and then join TableB and TableC.

# Output Format:
Please respond with XML code structured as follows.
<reasoning>
    Your detailed reasoning for the SQL query generation, with Recursive Divide-and-Conquer approach.
</reasoning>
<result>
    The final SQL query that answers the question and can be executed by SQLite directly, ensure there is not any SQLite comment and not any other explanation text in the SQL query.
    The SQL query must not include XML-specific characters (e.g., `&lt;`, `&gt;`, `&amp;`); only SQL-valid characters are allowed.
</result>

# Input:
## Database Schema:
{DATABASE_SCHEMA}

## Question:
{QUESTION}

## Hints:
{HINT}

Repeating the question and hint, and generating the SQL with Recursive Divide-and-Conquer approach, and finally try to simplify the SQL query using `INNER JOIN` over nested `SELECT` statements IF POSSIBLE.

# Output:
\end{lstlisting}

\clearpage
\subsection{ICL-based SQL Generation Prompt}
\label{subsec:prompt_icl_sql}

This prompt is for the \textit{ICL-based SQL Generator}. It leverages cross-domain few-shot examples to guide the LLM. The model is instructed to identify common patterns and logical structures from the provided question-SQL pairs and apply them to generate a query for the target question.

\begin{lstlisting}[
    frame=single,
    caption={ICL-based SQL Generation Prompt},
    label={lst:icl_sql},
    basicstyle=\ttfamily\small,
    breaklines=true
]
# Task:
You are an experienced database expert specializing in cross-domain SQL generation.
You will be given a target database schema, a question, and several similar examples from different databases (cross-domain few-shot examples).
Your task is to generate a SQL query for the target question by learning from the provided examples.

# Instructions:
1. **Analyze the Examples**: Study the provided few-shot examples carefully. Each example contains:
   - A question from a different database domain
   - The corresponding SQL query that answers the question

2. **Identify Patterns**: Look for common SQL patterns, query structures, and logical approaches used in the examples:
   - How to handle aggregations (MAX, MIN, COUNT, SUM, AVG)
   - How to structure JOINs and subqueries
   - How to apply WHERE conditions and filtering
   - How to handle string matching and comparisons
   - How to use ORDER BY and LIMIT clauses

3. **Apply to Target Question**: Use the learned patterns to generate SQL for the target question:
   - Map the target question's requirements to similar patterns from examples
   - Adapt the SQL structure to work with the target database schema
   - Ensure the query logic matches the question's intent

# Important Rules:
1. **Schema Adaptation**: The examples use different database schemas, so you must adapt the patterns to work with the target schema
2. **Column Mapping**: Pay attention to how similar concepts are represented in different schemas
3. **Query Structure**: Follow the structural patterns from examples (JOIN types, subquery usage, etc.)
4. **SQLite Compatibility**: Use only SQLite-compatible functions and syntax
5. **Exact Column Names**: Use the exact column and table names from the target schema
6. **Logical Consistency**: Ensure the generated query logically answers the target question
7. **Foreign Key Constraints**: If there are multiple tables to JOIN, you MUST ensure that the joined tables have EXPLICIT FOREIGN KEYS between them. For example, "TableA -> TableB, TableC -> TableB", directly join TableA and TableC is NOT ALLOWED, you must join TableA and TableB, and then join TableB and TableC.

# Output Format:
Please respond with XML code structured as follows:
<reasoning>
    Your analysis of the examples and reasoning for the SQL generation.
</reasoning>
<result>
    The final SQL query that answers the target question and can be executed on the target SQLite database, ensure there is not any SQLite comment and not any other explanation text in the SQL query.
    The SQL query must not include XML-specific characters (e.g., `&lt;`, `&gt;`, `&amp;`); only SQL-valid characters are allowed.
</result>

# Input:
## Few-Shot Examples:
{FEW_SHOT_EXAMPLES}

## Target Database Schema:
{DATABASE_SCHEMA}

## Target Question:
{QUESTION} {HINT}

# Output:
\end{lstlisting}

\clearpage
\subsection{Skeleton-based SQL Generation Prompt}
\label{subsec:prompt_skeleton_sql}

This prompt directs the \textit{Skeleton-based SQL Generator}. The LLM is instructed to follow a systematic three-step process: first, plan the query by analyzing the required SQL components; second, create a structured SQL skeleton with placeholders; and third, complete the skeleton to produce the final query.

\begin{lstlisting}[
    frame=single,
    caption={Skeleton-based SQL Generation Prompt},
    label={lst:skeleton_sql},
    basicstyle=\ttfamily\small,
    breaklines=true
]
# Task:
You are an expert SQL developer who uses a systematic approach to generate complex SQL queries.
Your task is to analyze the given question and database schema, then generate a SQL query using a three-step process:
1. **Plan**: Identify the required SQL components and logical structure
2. **Skeleton**: Create a structured SQL skeleton with placeholders
3. **Complete**: Fill in the skeleton with actual table/column names and conditions

# Instructions:

## Step 1: Plan (SQL Components Analysis)
Analyze the question and identify:
- **SELECT clause**: What data needs to be retrieved? (columns, aggregations, calculations)
- **FROM clause**: Which tables are needed?
- **JOIN clauses**: What relationships need to be established?
- **WHERE clause**: What filtering conditions are required?
- **GROUP BY clause**: What grouping is needed for aggregations?
- **HAVING clause**: What post-aggregation filtering is needed?
- **ORDER BY clause**: What sorting is required?
- **LIMIT clause**: Are there any row limits?
- **Subqueries**: Are nested queries needed?
- **Special functions**: Date functions, string functions, mathematical operations

## Step 2: Skeleton (Structured Template)
Create a SQL skeleton with:
- Clear structure showing the logical flow
- Placeholders for table names, column names, and conditions
- Comments explaining the purpose of each section
- Proper indentation and formatting

## Step 3: Complete (Final SQL)
Fill in the skeleton with:
- Exact table and column names from the schema
- Specific values and conditions from the question
- Proper SQLite syntax and functions
- Final validation of the query logic

# Important Rules:
1. **Schema Accuracy**: Use exact table and column names from the provided schema
2. **SQLite Compatibility**: Use only SQLite-compatible functions and syntax
3. **Logical Flow**: Ensure the query logic matches the question requirements
4. **Performance**: Prefer efficient JOIN patterns over nested subqueries when possible
5. **Readability**: Use clear aliases and proper formatting
6. **Completeness**: Address all aspects mentioned in the question and hint
7. **Foreign Key Constraints**: If there are multiple tables to JOIN, you MUST ensure that the joined tables have EXPLICIT FOREIGN KEYS between them. For example, "TableA -> TableB, TableC -> TableB", directly join TableA and TableC is NOT ALLOWED, you must join TableA and TableB, and then join TableB and TableC.


# Output Format:
Please respond with XML code structured as follows:
<reasoning>
    Your comprehensive analysis and planning for the SQL query generation and the SQL skeleton with placeholders.
</reasoning>
<result>
    The final SQL query that answers the target question and can be executed on the target SQLite database, ensure there is not any SQLite comment and not any other explanation text in the SQL query.
    The SQL query must not include XML-specific characters (e.g., `&lt;`, `&gt;`, `&amp;`); only SQL-valid characters are allowed.
</result>

# Input:
## Database Schema:
{DATABASE_SCHEMA}

## Question:
{QUESTION}

## Hint:
{HINT}

# Output:
\end{lstlisting}

\clearpage
\subsection{Execution-based Revision Prompt}
\label{subsec:prompt_execution_revision}

This prompt is used by checkers in the \textit{Tool-Chain} that rely on execution results, such as the `Syntax Checker' or `Result Checker'. When a query fails to execute or returns an empty/unexpected result, this prompt instructs the LLM to analyze the error message and the query's logic to provide a corrected version.

\begin{lstlisting}[
    frame=single,
    caption={Execution-based Revision Prompt},
    label={lst:execution_revision},
    basicstyle=\ttfamily\small,
    breaklines=true
]
# Task:
You are an SQL database expert tasked with correcting a SQL query. A previous attempt to run a query did not yield the correct results, either due to errors in execution or because the result returned was empty or unexpected. Your role is to analyze the error based on the provided database schema and the details of the failed execution, and then provide a corrected version of the SQL query.

# Instructions:
1. Review Database Schema:
    - Examine the database schema to understand the database structure.
2. Analyze Query Requirements:
    - Original Question: Consider what information the query is supposed to retrieve.
    - Hint: Use the provided hints to understand the relationships and conditions relevant to the query.
    - Executed SQL Query: Review the SQL query that was previously executed and led to an error or incorrect result.
    - Execution Result: Analyze the outcome of the executed query to identify why it failed (e.g., syntax errors, incorrect column references, logical mistakes).
3. Correct the Query: 
    - Modify the SQL query to address the identified issues, ensuring it correctly fetches the requested data according to the database schema and query requirements.
    - Use the retrieved values to help write more accurate conditions when appropriate.

[IMPORTANT]
For key phrases mentioned in the question, we have provided the most similar values within the columns (TEXT-TYPE columns) denoted by "Value Examples". **This is a critical hint to identify the tables/columns that will be used in the SQL query.**

# Output Format:
Please respond with XML code structured as follows.
<reasoning>
    Your detailed reasoning for the SQL query revision, including the detailed analysis of the previous query and the database schema, and try to fix the failed query.
</reasoning>
<result>
    The final revised SQL query that answers the question and can be executed by SQLite directly, ensure there is not any SQLite comment and not any other explanation text in the SQL query.
    The SQL query must not include XML-specific characters (e.g., `&lt;`, `&gt;`, `&amp;`); only SQL-valid characters are allowed.
</result>

# Input:
## Database Schema:
{DATABASE_SCHEMA}

## Question:
{QUESTION}

## Hint:
{HINT}

## Previous SQL:
{QUERY}

## Execution Result:
{RESULT}

Based on the question, table schemas, the previous query, and the execution result, analyze the result try to fix the query, and only output the XML code (<reasoning>...</reasoning> and <result>...</result>) as your response.

# Output:
\end{lstlisting}

\clearpage
\subsection{Rule-based Revision Prompt}
\label{subsec:prompt_common_revision}

This prompt is used by the rule-based checkers in the \textit{Tool-Chain} (\eg `JOIN Checker', `ORDER-BY Checker'). When a checker identifies a specific, non-execution-related flaw based on predefined rules, it generates a directive. This prompt then instructs the LLM to apply the suggested modification precisely.

\begin{lstlisting}[
    frame=single,
    caption={Rule-based Revision Prompt},
    label={lst:common_revision},
    basicstyle=\ttfamily\small,
    breaklines=true
]
# Task:
You are an SQL database expert tasked with correcting a SQL query. An external SQL checker tool has checked the SQL query and provided some suggestions to correct. Your role is to analyze the suggestions from the checker tool, and then based on the provided database schema provide a corrected version of the SQL query.

# Instructions:
1. Review Database Schema:
    - Examine the database schema to understand the database structure.
2. Analyze Query Requirements:
    - Original Question: Consider what information the query is supposed to retrieve.
    - Hint: Use the provided hints to understand the relationships and conditions relevant to the query.
    - SQL Query: Review the SQL query that was previously checked.
    - Modification Suggestions: Review the suggestions provided by the external checker, and think how to modify the SQL to meet the suggestions.
3. Correct the Query: 
    - Modify the SQL query based the given Modification Suggestions, ensuring it correctly meet the expected suggestions.
[IMPORTANT]
Your are NOT ALLOWED to do any other modifications which are not listed in given suggestions.
# Output Format:
Please respond with XML code structured as follows.
<reasoning>
    Your detailed reasoning for the SQL query revision, including understanding the given suggestions, analyzing of the previous query and database schema, and then try to fix the query.
</reasoning>
<result>
    The final revised SQL query that answers the question and can be executed by SQLite directly, ensure there is not any SQLite comment and not any other explanation text in the SQL query.
    The SQL query must not include XML-specific characters (e.g., `&lt;`, `&gt;`, `&amp;`); only SQL-valid characters are allowed.
</result>

# Input:
## Database Schema:
{DATABASE_SCHEMA}

## Question:
{QUESTION}

## Hint:
{HINT}

## Previous SQL:
{QUERY}

## Modification Suggestions:
{SUGGESTIONS}

Based on the question, database schemas, previous SQL query and modification suggestions, try to fix the query, and only output the XML code (<reasoning>...</reasoning> and <result>...</result>) as your response.

# Output:
\end{lstlisting}

\clearpage
\subsection{SQL Selection Prompt (Pairwise Adjudication)}
\label{subsec:prompt_selection}

This prompt is utilized in the \textit{Pairwise Adjudication} step of the \textit{Confidence-Aware SQL Selection} phase. It employs an \textit{Execution-Guided} strategy, where the LLM acts as a judge to compare two SQL candidates. The prompt explicitly introduces a bias towards the candidate with higher execution consensus (Candidate A), instructing the model to switch to Candidate B only if decisive logical evidence exists.

\begin{lstlisting}[
    frame=single,
    caption={SQL Selection Prompt (Pairwise Adjudication)},
    label={lst:sql_selection},
    basicstyle=\ttfamily\small,
    breaklines=true
]
# Task:
Given the DB info and question, there are two candidate queries. There is correct one and incorrect one, compare the two candidate answers, analyze the differences of the query and the result. Based on the original question and the provided database info, choose the correct one.

# Important Context:
- SQL Candidate A (Top-1) has higher confidence than SQL Candidate B (Top-2)
- SQL Candidate A's confidence was not high enough to meet the threshold, but it is still the more confident choice
- You should only choose SQL Candidate B if there is clear evidence that it is superior to SQL Candidate A, or if SQL Candidate A has obvious errors
- The default preference should be SQL Candidate A unless there are compelling reasons to choose SQL Candidate B
- If you cannot determine which SQL is better, or if both SQLs have significant issues, you should choose SQL Candidate A by default

# Instructions:
- Carefully analyze the user question, database schema, and both candidate SQL queries
- For each SQL, consider its logic, correctness, and the provided execution result
- Compare the two SQLs in terms of their ability to answer the question accurately and completely
- You can only select minimum columns requested by the user question
- Give preference to SQL Candidate A unless SQL Candidate B clearly demonstrates superiority or SQL Candidate A has obvious flaws
- In <result>, output 'A' or 'B' (just the letter/word):
  - 'A': SQL Candidate A is clearly better
  - 'B': SQL Candidate B is clearly better  

# Output Format:
Please respond with XML code structured as follows:
<result>
    A or B (just the letter/word)
</result>

# Input:
## Database Schema:
{DATABASE_SCHEMA}

## Question:
{QUESTION}

## Hint:
{HINT}

SQL Candidate A:
{QUERY_A}

## Execution Result:
{RESULT_A}

SQL Candidate B:
{QUERY_B}

## Execution Result:
{RESULT_B}

Based on the question and the two SQL queries, analyze which query answers the question correctly, and only output the XML code as your response.

# Output:
\end{lstlisting}
